# Supplementary material for: Exploring Long Tail Visual Relationship Recognition with Large Vocabulary
Source: arXiv:2004.00436 source file (2021-09-25)
Supplement: Supplementary file 1 [file appendix.tex]

\section*{Table of Contents}

\begin{enumerate}

\item Qualitative Examples
\item Implementation Details
\item Hyperparameters
\item Many, Medium, Few splits for GQA-LT and VG8K-LT
\item Object/Subject/Relationship class frequencies for GQA-LT and VG8K-LT
\item Human Subjects Experiment Setup
\item Motivation For Word2Vec and Wordnet Metrics
\item Additional Results on GQA-LT and VG8K-LT
\item Further discussion of RelMix Augmentation
\item Additional Results on VG200 (far more balanced than GQA-LT and VG8K-LT)
\item Further Analysis
\item Further Contrast with Related Work
\item Code (attached, includes implementation details) : \href{https://github.com/Vision-CAIR/LTVRR}{https://github.com/Vision-CAIR/LTVRR}
\item Video (attached, includes more qualitative examples) 
\item Dataset histograms that show the distribution of classes for subject, objects, and relations provided under "./histograms"
\item GQA-LT and VG8K-LT synsets to classes mapping:
   \begin{itemize}
    \item ./synsets\_mapping/gqa\_rel\_synset\_mapping.json 
    \item ./synsets\_mapping/gqa\_sbjobj\_synset\_mapping.json 
    \item ./synsets\_mapping/vg\_sbjobj\_synset\_mapping.json
    \item ./synsets\_mapping/vg\_rel\_synset\_mapping.json
   \end{itemize}
 
\end{enumerate}

\section{Qualitative Examples}
\begin{figure}[h!]
  \centering
  \includegraphics[width=0.9\linewidth]{AAAI_supp/figures/success_rel.png}
  \caption{A qualitative example showing how the model with the VilHub loss performs better on tail relation classes. Blue is subject, purple is relation, and orange is object. The left image is the LSVRU model, and the right image is LSVRU + ViLHub model}
\label{fig:success}
\end{figure}

\begin{figure}[h!]
  \centering
  \includegraphics[width=0.9\linewidth]{AAAI_supp/figures/success_relmix.png}
  \caption{A qualitative example showing how the model with the RelMix augmentation and VilHub loss performs better on tail relation classes. The left image is the LSVRU model, and the right image is LSVRU + RelMix + VilHub model}
\label{fig:success_relmix}
\end{figure}

\begin{figure}[h!]
  \centering
  \includegraphics[width=0.9\linewidth]{AAAI_supp/figures/failure_rel.png}   
  \caption{A qualitative example showing how the model with the VilHub sometimes fails by predicting a tail class instead of a head class. The left image is the LSVRU model, and the right image is LSVRU + ViLHub model}
\label{fig:failure}
\end{figure}

% \begin{figure*}[h!]
%   \centering
%   \includegraphics[width=\linewidth]{AAAI_supp/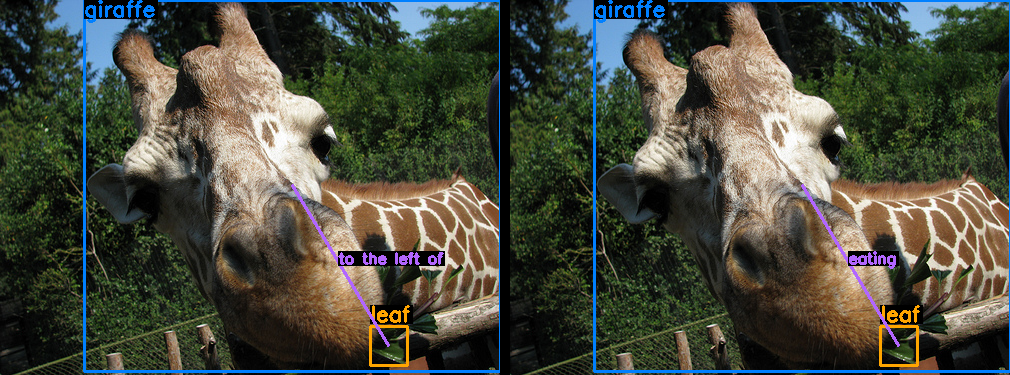}
%   \caption{A qualitative example showing how the model with the ViL-Hubless loss performs better on tail relation classes. Blue is subject, purple is relation, and orange is object. The left image is the LSVRU model, and the right image is LSVRU + ViLHub model}
% \label{fig:qual_rel}
% \end{figure*}

% \begin{figure*}[h!]
%   \centering
%   \includegraphics[width=\linewidth]{AAAI_supp/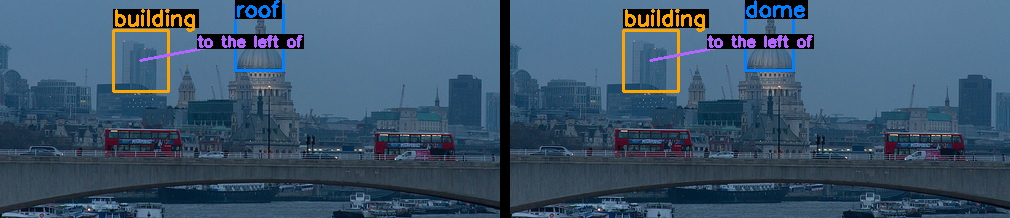}
%   \caption{A qualitative example showing how the model with the ViL-Hubless loss performs better on tail subject/object classes. Left image is the LSVRU model, and right image is LSVRU + ViLHub model}
% \label{fig:qual_sbj}
% \end{figure*}

Fig~\ref{fig:success} shows an example of one of the cases where the LSVRU model (left image) predicts a head class (\textit{to the left of}) that doesn't fit well while the LSVRU + VilHub model (right image) instead predicts a tail class (\textit{eating}) which is more accurate and descriptive in this case.

Similarly, Fig~\ref{fig:success_relmix} shows an example of one of the cases where the LSVRU model (left image) predicts a head class (\textit{to the right of}) that doesn't fit well while the LSVRU + RelMix + VilHub model (right image) instead predicts a tail class (\textit{holding}) which seems more suitable and descriptive for the particular triplet in question.

Fig~\ref{fig:failure} shows a failure case on the head, when the LSVRU + VilHub predicte a tail class while the correct class is a head class. More qualitative examples can be found in the attached video.

\section{Implementation Details}
% \begin{figure*}[h]
% \centering
% % \adjincludegraphics[width=\linewidth,trim={0 {.05\height} 0 0},clip]{fig/model.pdf}
% \includegraphics[width=0.8\linewidth]{AAAI_supp/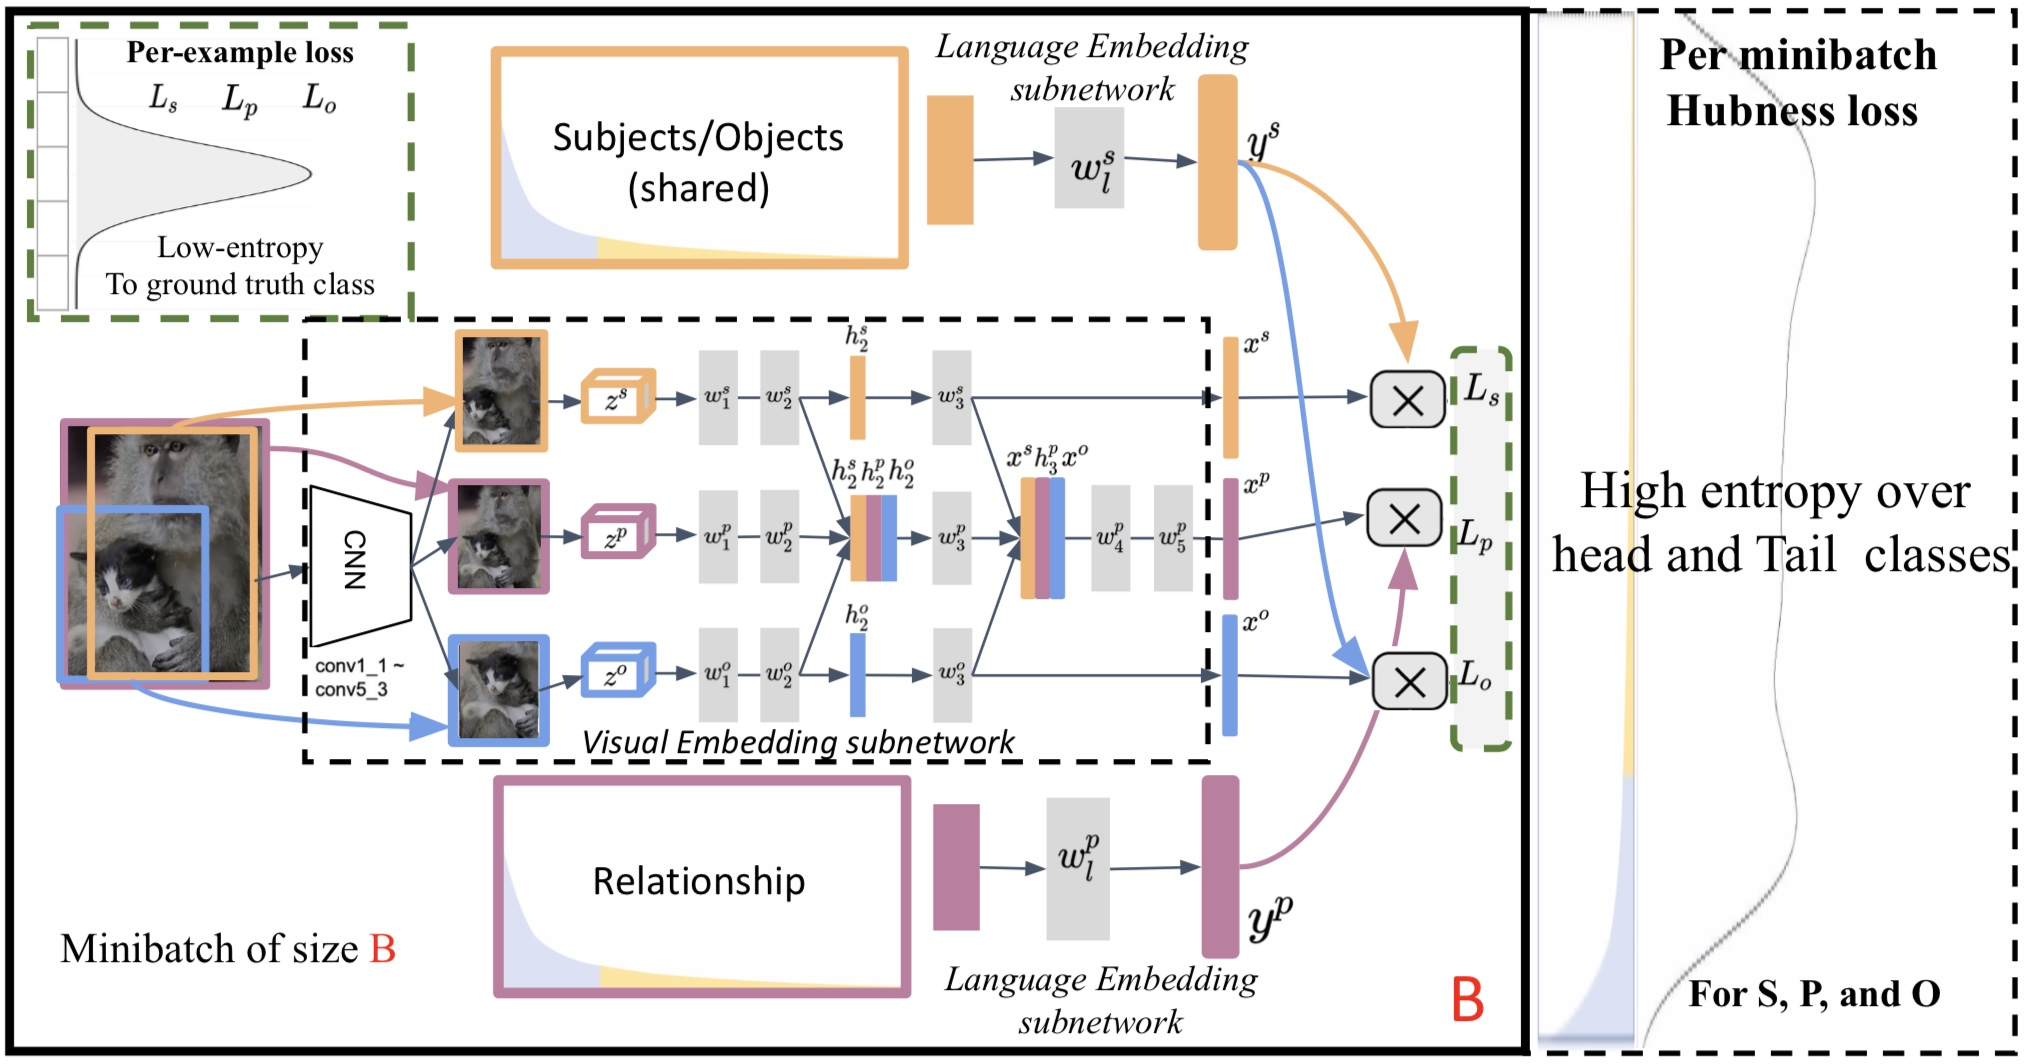}
% %\setlength\belowcaptionskip{-2ex}
% \captionsetup{font=small}
% \caption{\textbf{Main proposed architecture}. Our model is inspired from~\cite{zhang2019large} and it consists of a Visual Embedding Network and a Language Embedding Network. $L_s$, $L_p$, $L_o$ are per-example losses of subject, relation and object denoted here as \emph{low-entropy losses}. Orange, purple and blue colors represent subject, relation, object, respectively. The  layer weights of the subject and object branches are shared, \emph{\ie} $w^s_i$ and $w^o_i$, $i=1,2...5$. }
% \label{fig:model}
% \end{figure*}

% Fig~\ref{fig:model} shows our architecture, which builds on top of~\cite{zhang2019large}.

\noindent \textbf{Visual Embedding sub-network.} Similar to~\cite{plummerPLCLC2017,zhang2019large}, we learn embeddings for subject and object in a separate semantic space from the relation space. More concretely, we first get a global feature map of an input image processing in through a CNN ($conv1\_1$ to $conv5\_3$ of VGG16, then we perform  ROI-pooling of subject, relation and object features to get $z^s$, $z^p$, $z^o$ with the corresponding regions $\sregion$, $\pregion$, $\oregion$. Each branch followed by two fully connected layers which output three intermediate hidden features $h^s_2$, $h^p_2$, $h^o_2$. 
For the subject/object branch, a fully connected layer $w^s_3$ is added to get the visual embedding $x^s$, and similarly for the object branch to get $x^o$. Since we expect the network to recognition the object whether it appeared as as a subject or an object in a relationship, all the parameters of both branches are shared. 
Since  involving relation features for subject/object embeddings may undesirably entangling the two spaces, 
For the relation branch following~\cite{zhang2019large}, we apply an effective two-level feature fusion to finally  get the relation embedding $x^p$. 

\noindent \textbf{Language Embedding sub-network.}
On the language side, we feed word vectors of subject, relation and object labels into a two-layer neural network 
of one or two $fc$ layers which outputs the final embeddings. Similar to the visual module, we share subject and object branches share weights while the relation branch is unshared.
% ($w^s_l$ and $w^o_l$) are shared because both embeddings are in the same semantic space, while the relation branch ($w^p_l$) is independent. 
The purpose of this module is to map word vectors into an embedding space that is more discriminative than the raw word vector space while preserving semantic similarity. During training, we feed the ground-truth labels of each relationship triplet as well as labels of negative classes into the semantic module, as the following subsection describes; during testing, we feed the whole sets of object and relation labels into it for nearest neighbors searching among all the labels to get the top $k$ as our prediction.

\noindent\textbf{Language and Visual Context Word Embeddings.}
The language sub-network takes as an input skip-gram word Embeddings, which tries to maximize classification of a word based on another word in the same context. We performed experiments with two skip-gram models trained on language and visual contexts. The language word embedding model is provided by word2vec \cite{mikolov2013distributed}, pre-trained on Google News corpus as context.  The second \emph{visual word embedding model} is trained with the same loss of a skip-gram word2vec model where the context is defined as the training relationship instances. The optimization maximizes the  likelihoods of each relationship element given the other two (e.g., each of S, R, and O given SO, RO, SR, respectively). 

\section{Hyperparameters}
All models are trained with a base learning rate $LR = 0.01$ on 8 V100 gpus with a batch size of 1 image per batch and 512 boxes within a single image per batch. All models trained on GQA-LT were trained for 12 epochs, and all models trained on VG8K-LT were trained for 8 epochs. Models trained on GQA-LT were started with a random seed of 0 (for Numpy and Pytorch), and models trained on VG8K-LT were started with a seed of 3 (for Numpy and Pytorch). The train/val/test splits for both datasets are provided with the attached code.

\section{Many, Medium, Few splits for GQA-LT and VG8K-LT}
As discussed in the main paper, we split VG8K-LT data into \emph{many}, \emph{medium}, and \emph{few} shots based frequency percentiles, \emph{many}: top 5\% most frequent classes, \emph{medium}: middle 15\%, and \emph{few}: bottom 80\%. Here we will give details on the range of classes withing each split for both GQA-LT and VG8K-LT.\\
Tables \ref{gqa_split} and \ref{vg8k_split} shows the number of classes in various categories for GQA-LT and VG8K-LT respectively. The split is shown for both the training and testing data, and also the number of synsets in all the categories is also shown. For full splits and detailed information about this, please refer to the csv files under \emph{'./histograms'}, provided in the supplementary material.

% \noindent Subjects/Objects:\\
% \noindent \emph{few}: 2453 classes. frequencies from 1 to 686.\\
% \noindent \emph{medium}: 460 classes. frequencies from 688 to 5365.\\
% \noindent \emph{many}: 154 classes. frequencies from 5540 to 196944.\\

% \noindent Relations:\\
% \noindent \emph{few}: 1143 classes. frequencies from 4 to 182.\\
% \noindent \emph{medium}: 214 classes. frequencies from 182 to 1233.\\
% \noindent \emph{many}: 72 classes. frequencies from 1260 to 618687.\\

% \noindent Subjects/Objects:\\
% \noindent \emph{few}: 4264 classes. frequencies from 1 to 686.\\
% \noindent \emph{medium}: 799 classes. frequencies from 688 to 5365.\\
% \noindent \emph{many}: 267 classes. frequencies from 5540 to 196944.\\

% \noindent Relations:\\
% \noindent \emph{few}: 1600 classes. frequencies from 4 to 182.\\
% \noindent \emph{medium}: 300 classes. frequencies from 182 to 1233.\\
% \noindent \emph{many}: 100 classes. frequencies from 1260 to 618687.\\

\input{AAAI_supp/tables/gqa_many_med_few_split}
\input{AAAI_supp/tables/vg8k_many_med_few_split}

\section{Object/Subject/Relationship class frequencies for our GQA-LT and VG8K-LT Benchmarks}
\begin{figure}[h]
\centering
\begin{subfigure}{.3\textwidth}
%   \centering
  \includegraphics[width=\linewidth]{AAAI_supp/figures/gqa_sbj_hist_log.png}
%   \caption{}
  \label{fig:gqa_sbj_hist}
\end{subfigure}%
\begin{subfigure}{.3\textwidth}
%   \centering
  \includegraphics[width=\linewidth]{AAAI_supp/figures/gqa_rel_hist_log.png}
%   \caption{}
  \label{fig:gqa_rel_hist}
\end{subfigure}
\begin{subfigure}{.3\textwidth}
%   \centering
  \includegraphics[width=\linewidth]{AAAI_supp/figures/gqa_obj_hist_log.png}
%   \caption{}
  \label{fig:gqa_obj_hist}
\end{subfigure}
\begin{subfigure}{.3\textwidth}
%   \centering
  \includegraphics[width=\linewidth]{AAAI_supp/figures/vg8k_sbj_hist_log.png}
%   \caption{}
  \label{fig:vg_sbj_hist}
\end{subfigure}%
\begin{subfigure}{.3\textwidth}
%   \centering
  \includegraphics[width=\linewidth]{AAAI_supp/figures/vg8k_rel_hist_log.png}
%   \caption{}
  \label{fig:vg_rel_hist}
\end{subfigure}
\begin{subfigure}{.3\textwidth}
%   \centering
  \includegraphics[width=\linewidth]{AAAI_supp/figures/vg8k_obj_hist_log.png}
%   \caption{}
  \label{fig:vg_obj_hist}
\end{subfigure}

\caption{The histograms showing the sbj, rel, obj frequencies for the GQA-LT and VG8K-LT dataset. The figures shows the frequency values in log scale. The actual frequencies for each class are attach in csv format.}
\label{fig:dataset_hist}
\end{figure}

The Fig~\ref{fig:dataset_hist} shows the Subject, Object, Relationship class frequencies for GQA-LT and VG8K dataset. While the values here shown in graphs are in log scale, the frequencies for sbj/obj/rel for both of the dataset can be found in the code folders provided alongside the supplementary submission.

\section{Human Subjects Experiment Setup.}
%The conclusion that the ground truth as a metric is too harsh and might not give us the whole picture of the models' performance was based on intuition and observations from the training data. 
%To confirm our intuition that the ground truth is too harsh we performed a human subjects experiment to evaluate the efficacy/harshness of the ground truth as a metric. 
We randomly selected 100 examples from Visual Genome dataset~\cite{krishna2017visual} and evaluated 5 hypotheses for each. Out of these 5 hypotheses, 1 was the Ground Truth (GT) and the other 4 were top predictions from~\cite{zhang2019large} excluding GT. In this experiment we had 3 human subjects, who were asked to evaluate each hypothesis from a scale of 1 to 5, 1 being the worst and 5 the best. The human subjects were blind to which hypothesis was the ground truth and which were a prediction by the model~\cite{zhang2019large}. Afterward we created a new ground truth from the majority voting of the 3 subjects and the ground truth on each example, we call this new ground truth Human-GT.

% \begin{figure}[t!] %todo remove our names from figures
%   \centering
%   \includegraphics[width=.4\linewidth]{AAAI_supp/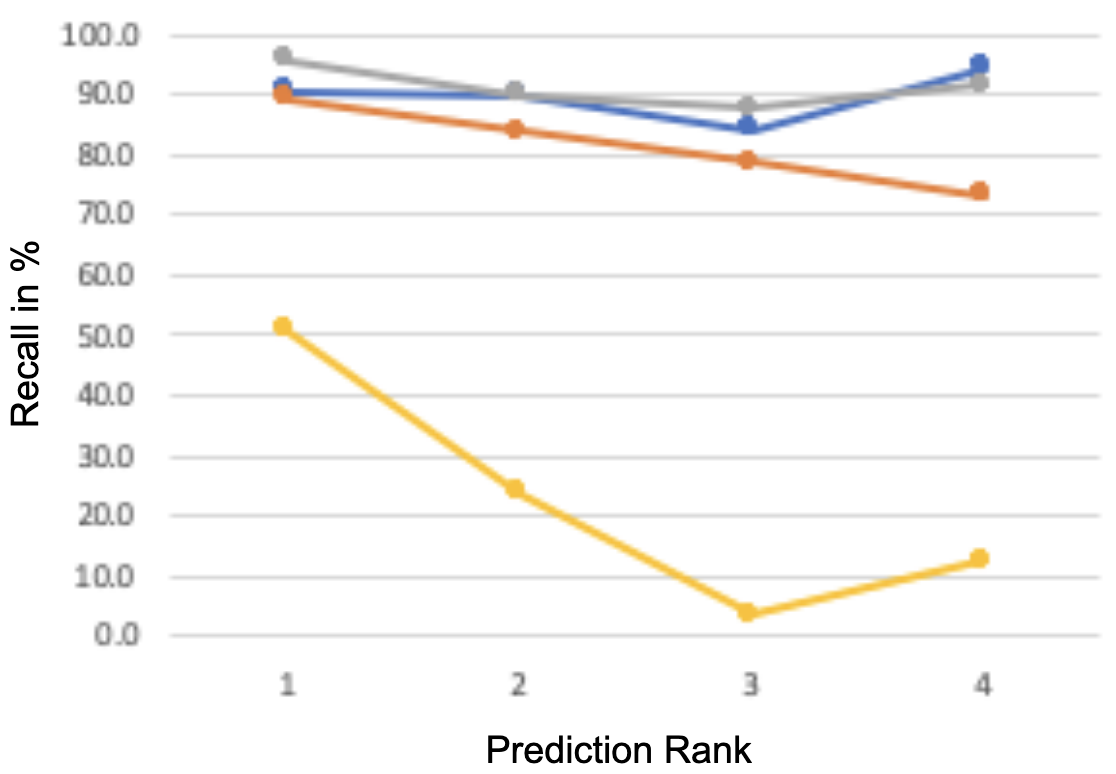}
%   \label{fig:recall}
% \caption{Recall scores of each of the human subjects (\textcolor{mygray}{gray}, \textcolor{blue}{blue}, \textcolor{red}{red}) and the ground truth (\textcolor{gold_web}{\textbf{gold}}) against the Human-GT}
% \vspace{-4mm}
% \label{fig:human_gt}
% \end{figure}
%Fig~\ref{fig:humansbj_exp} shows a human subject experiment that motivates an analysis methodology that we propose here to analyze different methods based on WordNet and word2vec.  We chose randomly 100 visual relationship validation examples and evaluated 5 hypotheses for each; Ground Truth (GT) and the top 4 predictions by~\cite{zhang2019large} excluding GT. Hence, we collected a total of 500  responses from human subjects ranging from 1 (awful) to 5 (excellent).  We tried both Mechanical Turk~\cite{buhrmester2011amazon} and graduate students in the  AI field and we observed better consistency and inter-rater agreement within  AI researchers,  measured with Cohen's Kappa score~\cite{cohen1960coefficient}, and hence we focus on them here\footnote{The inner annotator analysis for AI researchers vs Turkers can be found in the supplementary}.
We then computed the precision and recall of each of the human subjects and the ground truth against the Human-GT and we show the recall and precision in Fig~\ref{fig:prec_rec_human_gt}. If we look at Fig~\ref{fig:prec_rec_human_gt} we can see that the ground truth has a very low recall compared with the human subjects. This implies that a very large percentage of the hypotheses labeled as incorrect by the ground truth is, in fact, correct (high number of false negatives). This confirms our suspicion that the GT on its own is not sufficient to gain a deep understanding of how the models are performing on this problem. Note, because the gap in recall between the GT and human subjects was large enough, 100 random examples are enough to reach confidence level of 99.73\%. 
We did not observe a difference in precision between the human subjects and the GT. This implies is that the labels that GT labels as correct are also considered correct by the Human-GT (low number of false positives).

\section{Motivation For Word2Vec and Wordnet Metrics}
\label{sec_appendix_motivation}
The ground truth by construction assumes that there is one and only one right answer. Fig~\ref{fig:metric_motive_exp} shows an example of such case. In this case, the top 5 predictions from the model are all correct and very plausible. It's very hard to say any of these are wrong. There are many examples as the one in Fig~\ref{fig:metric_motive_exp} throughout the 2 datasets (GQA-LT and VG8K-LT). This illustrates that the ground truth with only one correct answer is fundamentally flawed for this task, and this is the motivation behind our proposed metrics.

\begin{figure}
\centering
\begin{subfigure}{.49\linewidth}
\includegraphics[width=\linewidth]{AAAI_supp/figures/recall.png}
\label{fig:rec_human_gt}
\end{subfigure}
\begin{subfigure}{.49\linewidth}
\centering
\includegraphics[width=\linewidth]{AAAI_supp/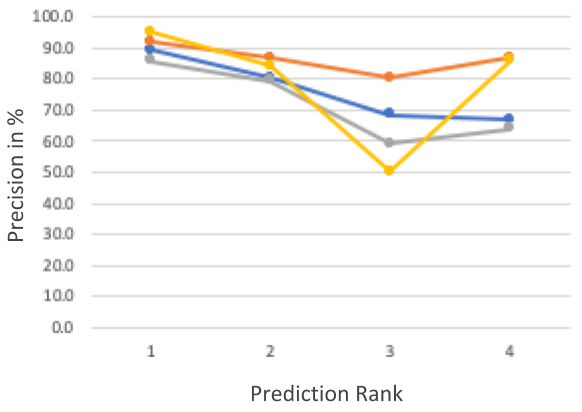}
\label{fig:prec_human_gt}
\end{subfigure}
\caption{Precision and Recall scores of each of the human subjects (gray, blue, red) and the ground truth (gold) against the Human-GT}
\label{fig:prec_rec_human_gt}
\end{figure}

\begin{figure}[ht!]
\centering
 \includegraphics[width=.3\textwidth]{AAAI_supp/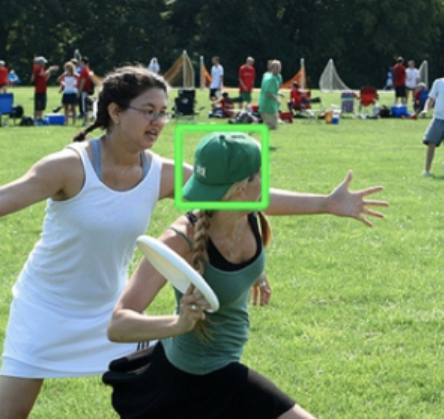}
  \caption{\textbf{This example is meant to show how some boxes can have multiple good answers}. The top 5 predictions for the above box ares: [Baseball Cap, Cap, Green Hat, Hat, Head]. This shows how it is unreasonable to evaluate this task assuming there is only one correct answer.}
\label{fig:metric_motive_exp}
\end{figure}

\section{Additional Results on GQA-LT and VG8K-LT}

\begin{table}
\centering
\caption{\label{tab:gvqa_triplets}Triplet Scores on GQA using Synsets}
\scalebox{0.7}
{
\begin{tabular}{lrrrr}
\toprule
Model &  many &  median &   few &   all \\
\midrule
\cite{zhang2019large}                   &  42.8 &    25.8 &   9.0 &  13.2 \\
\cite{zhang2019large} + ViLHub 10k      &  43.5 &    27.5 &   9.7 &  14.1 \\
\Delta                                  &   \bf+0.7 &     \bf+1.7 &   \bf+0.7 &   \bf+0.9 \\
\midrule
FL~\cite{lin2017focal}                  &  43.2 &    27.5 &   9.7 &  14.1 \\
FL + ViLHub                             &  44.4 &    29.8 &  11.5 &  15.9 \\
\Delta                                  &   \bf+1.2 &     \bf+2.3 &   \bf+1.8 &   \bf+1.8 \\
\midrule
WCE                                     &  19.4 &    14.8 &   7.6 &   9.2 \\
WCE + ViLHub                            &  18.0 &    14.8 &   7.9 &   9.4 \\
\Delta                                  &  \bf-1.4 &     \bf0.0 &   \bf+0.3 &   \bf+0.2 \\
\midrule
FC                                      &  39.2 &    20.4 &   6.3 &  10.0 \\
FC + ViLHub                             &  41.8 &    23.4 &   7.3 &  11.5 \\
\Delta                                  &   \bf+2.6 &     \bf+3.0 &   \bf+1.0 &   \bf+1.5 \\
\midrule
DCPL~\cite{Kang2020Decoupling}          &  33.7 &    20.2 &   7.3 &  10.6 \\
DCPL + ViLHub                           &  29.3 &    19.6 &   7.8 &  10.6 \\
\Delta                                  &  \bf-4.4 &    \bf-0.6 &   \bf+0.5 &   \bf0.0 \\
\midrule
OLTR                                    &  42.6 &    26.0 &   9.1 &  13.3 \\
EQL                                     &  44.4 &    30.0 &  11.7 &  16.0 \\
\bottomrule
\end{tabular}
}
\end{table}
\begin{table}
\centering
\caption{\label{tab:vg8k_triplets}Triplet Scores on VG8K using Synsets}
\scalebox{0.7}
{
\begin{tabular}{lrrrr}
\toprule
{} &  many &  median &  few &  all \\
\midrule
\cite{zhang2019large}                   &  24.0 &    10.1 &  3.1 &  5.2 \\
\cite{zhang2019large} + ViLHub 20k      &  21.6 &     7.3 &  4.3 &  5.6 \\
\Delta                                  &   \bf+0.8 &     \bf+0.5 &  \bf+0.2 &  \bf+0.3 \\
\midrule
WCE                                     &  10.1 &     4.4 &  2.8 &  3.4 \\
WCE + ViLHub                            &   9.2 &     4.1 &  2.7 &  3.3 \\
\Delta                                  &  \bf-0.9 &    \bf-0.3 & \bf-0.1 & \bf-0.1 \\
\midrule
FL~\cite{lin2017focal}                  &  15.1 &     6.1 &  4.0 &  4.9 \\
DCPL~\cite{Kang2020Decoupling}          &  14.5 &     5.5 &  2.8 &  3.8 \\
\bottomrule
\end{tabular}
}
\end{table}

\begin{table}[ht!]
\centering
\caption{\label{tab:per_class_wordsim} Per-class word similarity on subjects/objects in GQA}
\scalebox{0.8}
{
\begin{tabular}{l|ccccc}
\toprule
% {}              & \multicolumn{5}{c|}{sbj/obj}  \\
% \midrule
Models &  lch &  wup &  lin &  path &  w2v  \\
\midrule
Baseline~\cite{zhang2019large}                        &     51.2 &     59.4 &     36.8 &      27.5 &     45.2  \\
Baseline + ViLHub 10k           &     52.0 &     60.1 &     37.8 &      28.6 &     45.8  \\
Baseline + ViLHub 50k           &     53.1 &     61.0 &     39.0 &      30.1 &     46.7  \\
Baseline + ViLHub 100k          &     \bf53.4 &     \bf61.3 &     \bf39.5 &      \bf30.6 &     \bf47.1  \\
\midrule
FL~\cite{lin2017focal}                              &     51.8 &     60.0 &     37.5 &      28.3 &     45.7  \\
FL + ViLHub20k                  &     \bf53.2 &     \bf61.1 &     \bf39.1 &      \bf30.3 &     \bf47.0  \\
\midrule
WCE                             &     53.5 &     61.1 &     39.4 &      31.8 &     47.8  \\
WCE + ViLHub                    &     \bf54.8 &     \bf62.1 &     \bf41.0 &      \bf33.5 &     \bf49.2  \\
\midrule
FC                              &     48.9 &     57.1 &     33.8 &      24.5 &     43.3  \\
DCPL$_\tau$~\cite{Kang2020Decoupling}                     &     49.0 &     57.3 &     33.9 &      24.5 &     43.2  \\
DCPL$_m$~\cite{Kang2020Decoupling}                        &     49.1 &     57.4 &     34.1 &      25.8 &     43.0  \\
DCPL$_m$ + ViLHub100k           &     \bf50.4 &     \bf58.4 &     \bf35.5 &      \bf27.3 &     \bf44.7  \\
\bottomrule
\end{tabular}
}
\end{table}

% &     52.1
% &     51.8
% &     51.4
% &     51.3
% &     51.7
% &     51.4
% &     47.4
% &     46.7
% &     51.6
% &     51.6
% &     50.5
% &     48.7
\input{AAAI_supp/tables/gqa_variance_many_median_few_syn}
\input{AAAI_supp/tables/gqa_triplet_acc_many_med_few}
% \input{AAAI_supp/tables/vg200_results}

% We showed that the GT is not sufficient on its own to evaluate a model's performance, so calculated the metrics using synset matching. This means that if the wordnet synset of the prediction matches the wordnet synset of the GT this counts as a correct prediction. We show the metrics calculated using this approach in table~\ref{tab:many_medium_few_syn}. We can see that the same pattern of adding ViL-Hubless Loss improves performance on the medium and few classes but with higher numbers overall for all the models.
Table~\ref{tab:gqa_variance} shows some of the main models from the paper on GQA-LT dataset. The scores shown in Table~\ref{tab:gqa_variance} are calculated over several runs for each model (between 2 and 3 runs) and the mean and confidence intervals (calculated at confidence=95\%) are reported. The table shows that most improvement are outside the margin of error. This further strengthens our confidence in the results reported in the main paper.
In Table~\ref{tab:per_class_wordsim} shows the average per-class word similarity measured through wordnet and word2vec metrics for the subject and object categories. We can see the pattern more consistently here, where the models with the VilHub loss added have higher average per-class word similarity to the ground truth.

Table~\ref{tab:gvqa_triplets} and~\ref{tab:vg8k_triplets} show the performance on subject, relation, object (SRO) triplets scores on GQA-LT and VG8K-LT, respectively. An SRO triplet prediction is considered correct if the prediction for the subject, object, and relation are all correct. We separate the SRO triplets into few, medium, and many shots based on how many times the SRO triplet occures in the training data. As we did with the subject/object and relation tables in the main paper, we determine many, medium, few shots based on frequency percentile. (many: top 5\% most frequent, medium: middle 15\%, and few: bottom 80\%).
Table~\ref{tab:gvqa_triplets} and~\ref{tab:vg8k_triplets} show that adding the VilHub loss and RelMix augmentation increases the performance on almost all the cases.

Tables~\ref{tab:triplet_many}, \ref{tab:triplet_med} and \ref{tab:triplet_few} show the compositional results (the results when grouped by SO, SR and OR) on many, med and few categories respectively. In all these, we see a clear gain when adding VilHub \& RelMix on top of various base models.
% Table~\ref{tab:vg_many_medium_few} shows a similar patterns to the table in the main paper. Adding the ViLHub loss seems to improve performance on tail classes, without hurting the head performance and sometimes improving it. It seems that the higher the number of classes the higher the hubness scale needed, this is observed from how the relationships benefit from small hubness scale while the subjects and objects benefit much more from high hubness scales. This is explored further in Fig~\ref{fig:appendix_trends}

\clearpage

\section{Further discussion of RelMix Augmentation}

\input{AAAI_supp/tables/relmix_ablation}

In Table~\ref{tab:relmix_ablation}, we evaluate RelMix performance when different proportions ($\eta = 30\%, 50\%, 70\%$) of augmented data (w.r.t the original training size) is added to the original data mix. As can be seen from Table~\ref{tab:relmix_ablation}, we see slightly better results for $\eta = 50\%$ as compared to other proportions. Apart from this as we increase the augmentation proportion we see a slight gain in training time because of the increment in training data (original + augmented). Taking all this in account, we chose $\eta = 50\%$ for all the experimental results mentioned in Table 1\&2 in the main paper. 

\textbf{Choice of $\lambda$ in Eq.6 in main paper: } We validate various values for our mixing parameter $\lambda$ ranging from $0.5 - 0.9$ and also try random value assignment within the range. We obtain the optimal results on tail classes being when $\lambda$ is in the range $0.7 - 0.8$, with the difference being of approximately $0.5\%$ in the $few$ category and $0.3\%$ overall. This is since  a bigger $\lambda$  value leads to higher percentage of features from $\textbf{x}_i$ augmented from tail categories.

\section{Additional Results on VG200 (far more balanced than GQA-LT and VG8K-LT)}

\input{AAAI_supp/tables/vg200_results}

We also evaluate the performance of our proposed VilHub loss with RelMix augmentation on VG200 dataset. It contains most frequent 150 objects and 50 relations, and each category frequency in this dataset is considerably more balanced than in GQA-LT and VG8K-LT. We follow the same data split as in \cite{zhang2019large}.
Table~\ref{vg200_result} shows the performance of our model on top of LSVRU when evaluated on VG200. As can be clearly seen, the proposed VilHub+RelMix does not deteriorate the base model's performance on both the metrices (SGCLS and PRDCLS) and even manages to slightly improve upon it. However, a thing to keep in mind here is that our model manages to make the final prediction much more balanced (as can be seen from Table 1 and 2 in the paper) while not deteriorating the performance on these standard metrices (which are inherently much more biased towards \emph{head} class classification).

\section{Further Analysis}
\label{sec_appendix_analysis}
% \begin{figure}[!t]
%   \centering
% %   \vspace{-20mm}
% \begin{subfigure}{.45\textwidth}
%   \centering
%   \includegraphics[width=\linewidth]{AAAI_supp/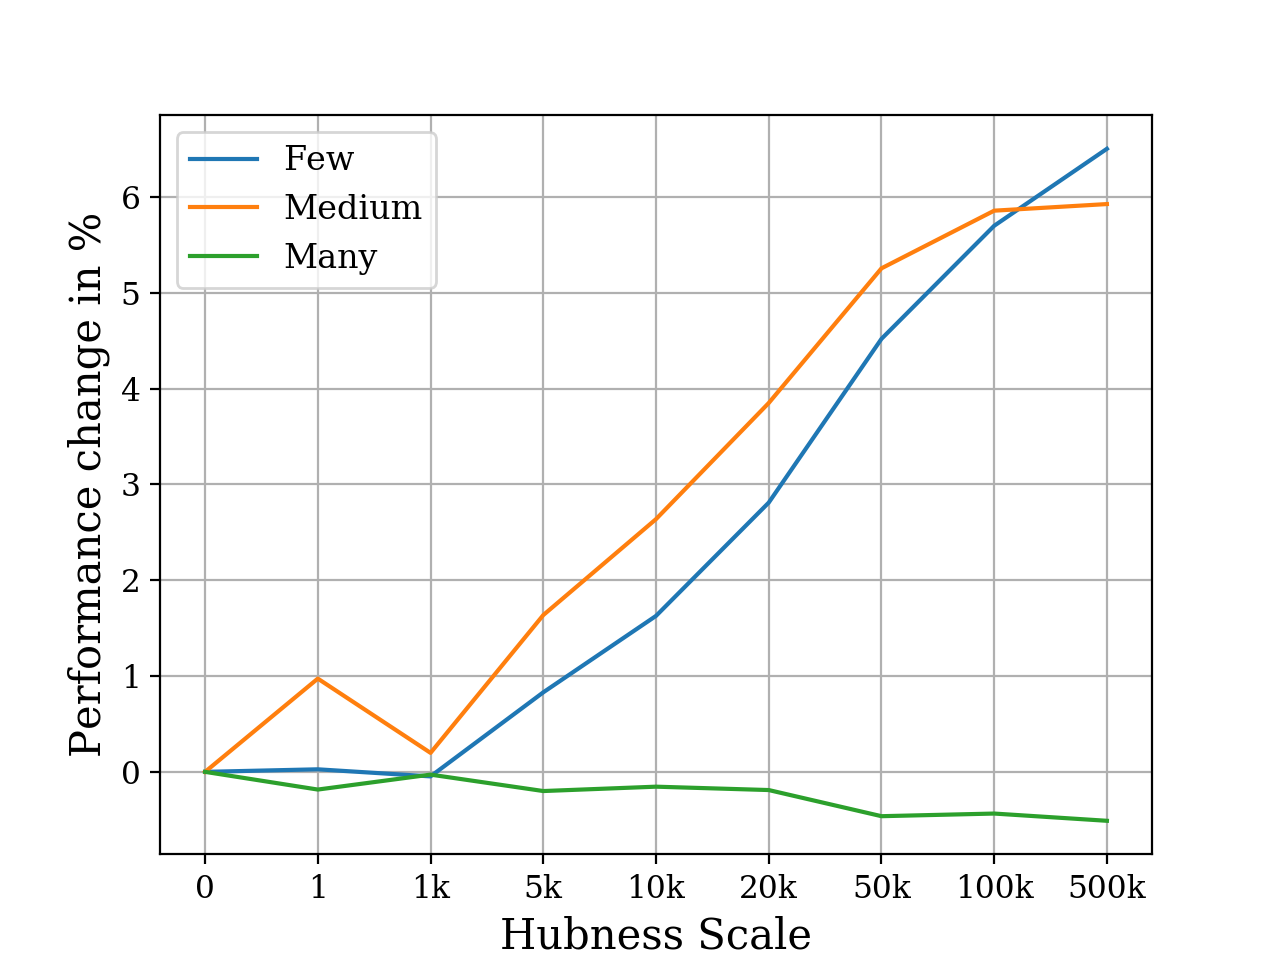}
%   \caption{Trend on subjects/objects}
%   \label{fig:sbj_trend}
% \end{subfigure}
% \begin{subfigure}{.45\textwidth}
%   \centering
%   \includegraphics[width=\linewidth]{AAAI_supp/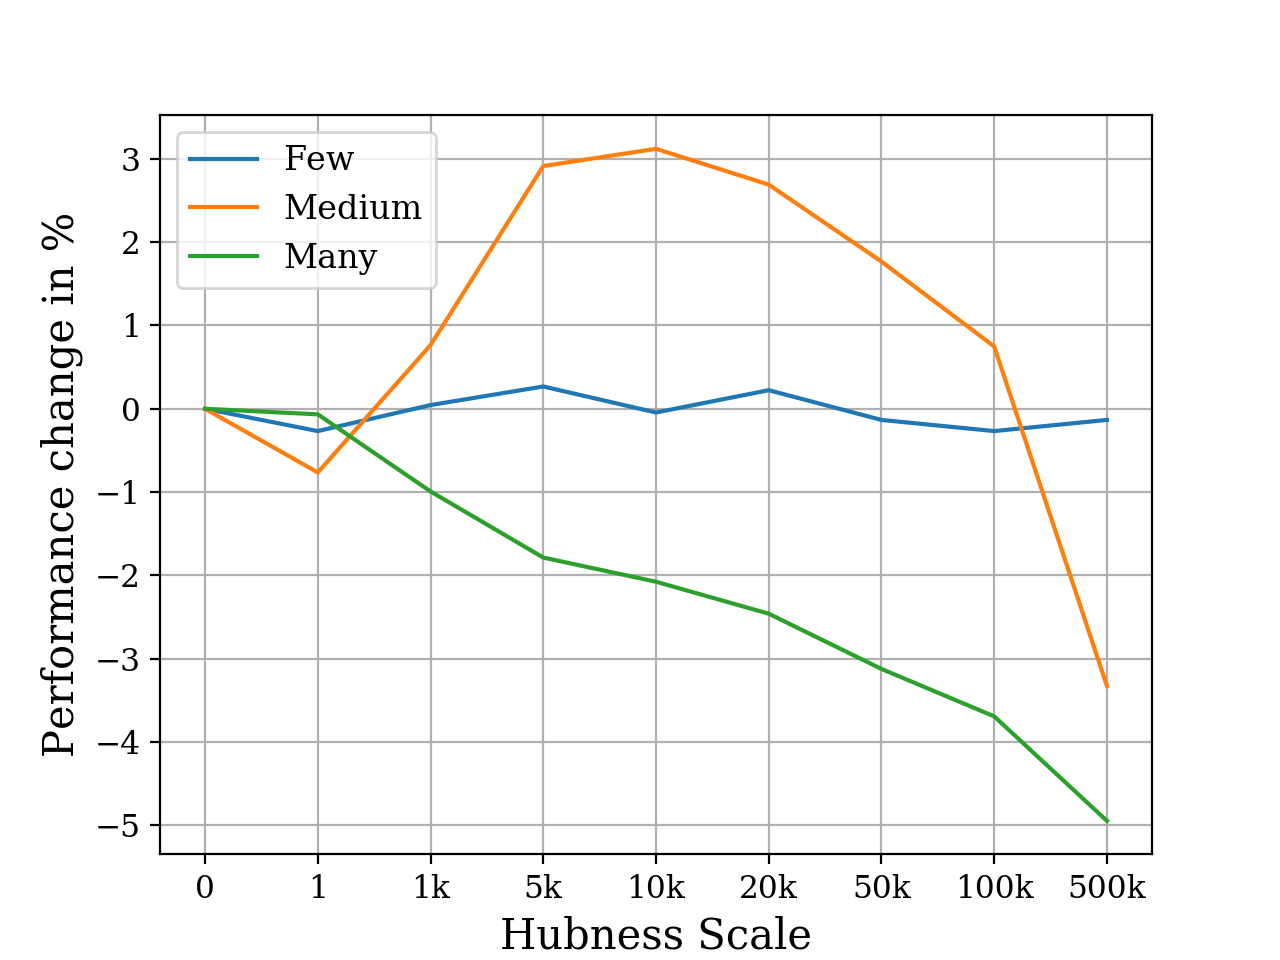}
%   \caption{Trend on relations}
%   \label{fig:rel_trend}
% \end{subfigure}
% \caption{This is a similar version to the figures shown in the main paper, tested with more ViL-Hubless scales. The figure shows how the performance changes on the many, medium, few parts of the classes as we increase the ViL-Hubless scale. Many: most frequent 5\% of classes, Medium: 20\% to 5\% most frequent, Few: least frequent 80\% of classes}
% \label{fig:appendix_trends}
% \end{figure}

% From Fig~\ref{fig:appendix_trends} we can see that as we increase the ViL-Hubless scale, the performance improves on the medium and few classes (tail) for subjects and objects. However for the relations, the optimal ViL-Hubless scale seems to lie somewhere around 10k, if we increase the scale further the performance starts to drop significantly. More experimentation is needed to determine the exact optimal value for VilHub scale for subjects/objects and relations.
 
Figure~\ref{fig:comps_gqa} shows the same comparision done in the main paper in Figure 4, but for several other models, comparing the results with and without using the VilHub loss. We can observe that the same pattern of improving the performance on \emph{medium} and \emph{few} shots seen in the main paper still holds true for other models. The only exception is the performance on relationships for DCPL vs DCPL + VilHub, where we see classes worsening on the \emph{few} category. However, VilHub loss still shows performance improvement on the \emph{medium} category.

\begin{figure}[h]
\begin{subfigure}{\textwidth}
\centering
\includegraphics[width=0.7\linewidth]{AAAI_supp/figures/comparisons/vg_baseline_vs_hub100k_sbj_syn.pdf}
\end{subfigure}
\begin{subfigure}{\textwidth}
\centering
\includegraphics[width=0.7\linewidth]{AAAI_supp/figures/comparisons/vg_baseline_vs_hub10k_rel_syn.pdf}
\caption{LSVRU vs. LSVRU + ViLHub for S/O (upper) and R (lower) on VG8K-LT}
\end{subfigure}
\caption{Comparisons of subject/object (upper) and relations (lower) performances between LSVRU model with and without ViLHub on VG8K-LT dataset. Note that the number of classes is slightly less than the listed number of classes for VG8K-LT, this is because these are the classes present in the test set only.}
\label{fig:comps_vg}
\end{figure}

Figure~\ref{fig:comps_vg} shows the comparision between LSVRU vs LSVRU + VilHub for VG8K-LT dataset. We can see that adding the VilHub improves performance on the \emph{medium} and \emph{few} categories, as it did on GQA-LT.

\begin{figure}
\begin{subfigure}{1.0\linewidth}
\centering
\includegraphics[width=0.7\linewidth]{AAAI_supp/figures/comparisons/fl_vs_fl_hub20k_sbj_syn.png}
\end{subfigure}
\begin{subfigure}{\linewidth}
\centering
\includegraphics[width=.7\linewidth]{AAAI_supp/figures/comparisons/fl_vs_fl_hub20k_rel_syn.png}
\caption{FL vs. FL + ViLHub for S/O (upper) and R (lower) on GQA-LT}
\end{subfigure}
% \begin{subfigure}{\linewidth}
% \centering
% \includegraphics[width=.7\linewidth]{AAAI_supp/figures/comparisons/fc_vs_fc_hub100k_sbj_syn.png}
% \end{subfigure}
% \begin{subfigure}{\linewidth}
% \centering
% \includegraphics[width=.7\linewidth]{AAAI_supp/figures/comparisons/fc_vs_fc_hub100k_rel_syn.png}
% \caption{FC vs. FC + ViLHub for S/O (upper) and R (lower) on GQA-LT}
% \end{subfigure}
\begin{subfigure}{\linewidth}
\centering
\includegraphics[width=0.7\linewidth]{AAAI_supp/figures/comparisons/dcpl_vs_dcpl_hub100k_sbj_syn.png}
\end{subfigure}
\begin{subfigure}{\linewidth}
\centering
\includegraphics[width=0.7\linewidth]{AAAI_supp/figures/comparisons/dcpl_vs_dcpl_hub100k_rel_syn.png}
\caption{DCPL vs. DCPL + ViLHub for S/O (upper) and R (lower) on GQA-LT}
\end{subfigure}
\caption{Comparisons of subject/object (upper) and relations (lower) performances between several models with and without ViLHub on GQA-LT dataset. We report the performance for all classes sorted by frequency. The distribution of classes for both figures is shown in the background. Note that the number of classes is slightly less than the listed number of classes for GQA-LT, this is because these are the classes present in the test set only.}
\label{fig:comps_gqa}
\end{figure}

Figure~\ref{fig:avg_prec_gn} shows the average precision metric on the tail for W2V trained on Google News (W2V-GN). It shows the same patterns as in Figure 5 in the main paper. Note that the scores using W2V-GN is less than when using W2V-VG. This is because W2V-VG is trained on more a relevant data to the task (Visual Genome) than W2V-GN.

\begin{figure}
\centering
\begin{subfigure}{\textwidth}
  \centering
  \includegraphics[width=.8\linewidth]{AAAI_supp/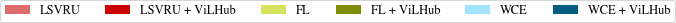}
\end{subfigure}
\begin{subfigure}{.3\textwidth}
  \centering
  \includegraphics[width=\linewidth]{AAAI_supp/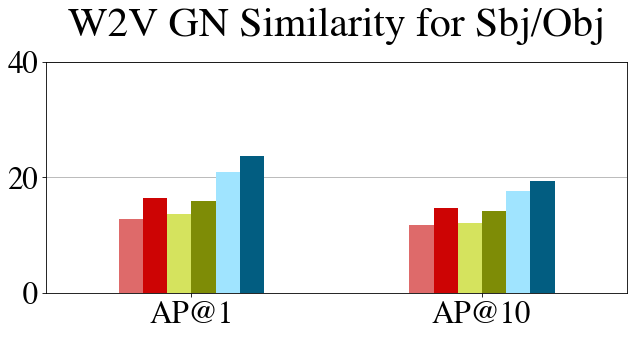}
  \caption{}
  \label{fig:avg_prec2}
\end{subfigure}%
\begin{subfigure}{.3\textwidth}
  \centering
  \includegraphics[width=\linewidth]{AAAI_supp/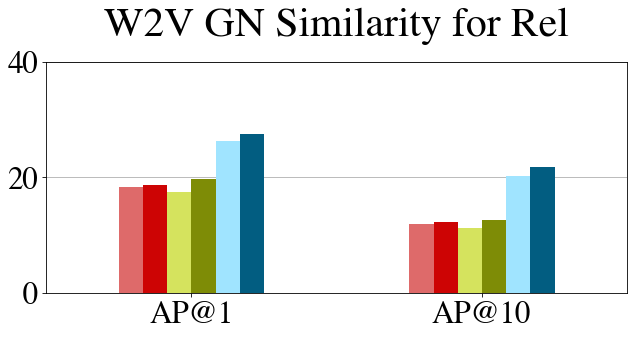}
  \caption{}
  \label{fig:avg_prec2}
\end{subfigure}%
\caption{\textbf{Average precision analysis on the tail classes (lower 80\% on GQA-LT dataset using a variety of metrics.} calculated using W2V trained Google News, showing the same pattern as the figures in the main paper}
\label{fig:avg_prec_gn}
\end{figure}

\begin{figure}[h]
\centering
\begin{subfigure}{\textwidth}
  \centering
  \includegraphics[width=.8\linewidth]{AAAI_supp/figures/average_precision_tail/legend.png}
\end{subfigure}
\begin{subfigure}{.3\textwidth}
%   \centering
  \includegraphics[width=\linewidth]{AAAI_supp/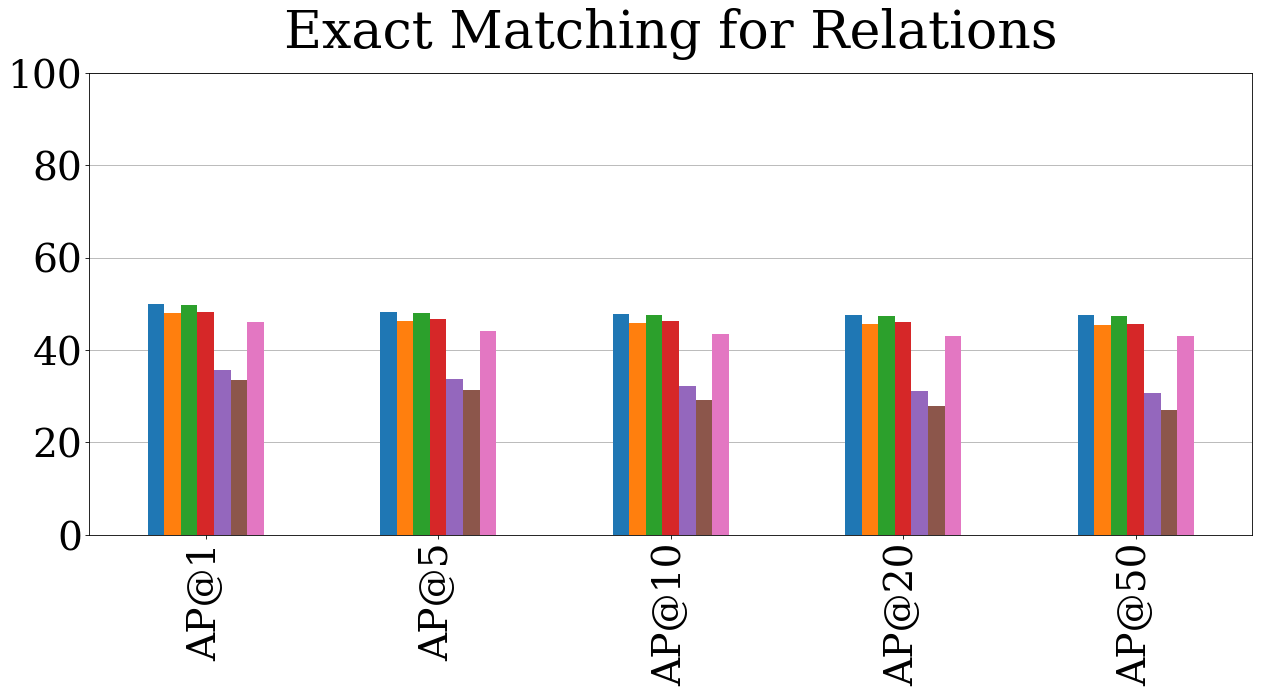}
%   \caption{}
  \label{fig:avg_prec1}
\end{subfigure}%
\begin{subfigure}{.3\textwidth}
%   \centering
  \includegraphics[width=\linewidth]{AAAI_supp/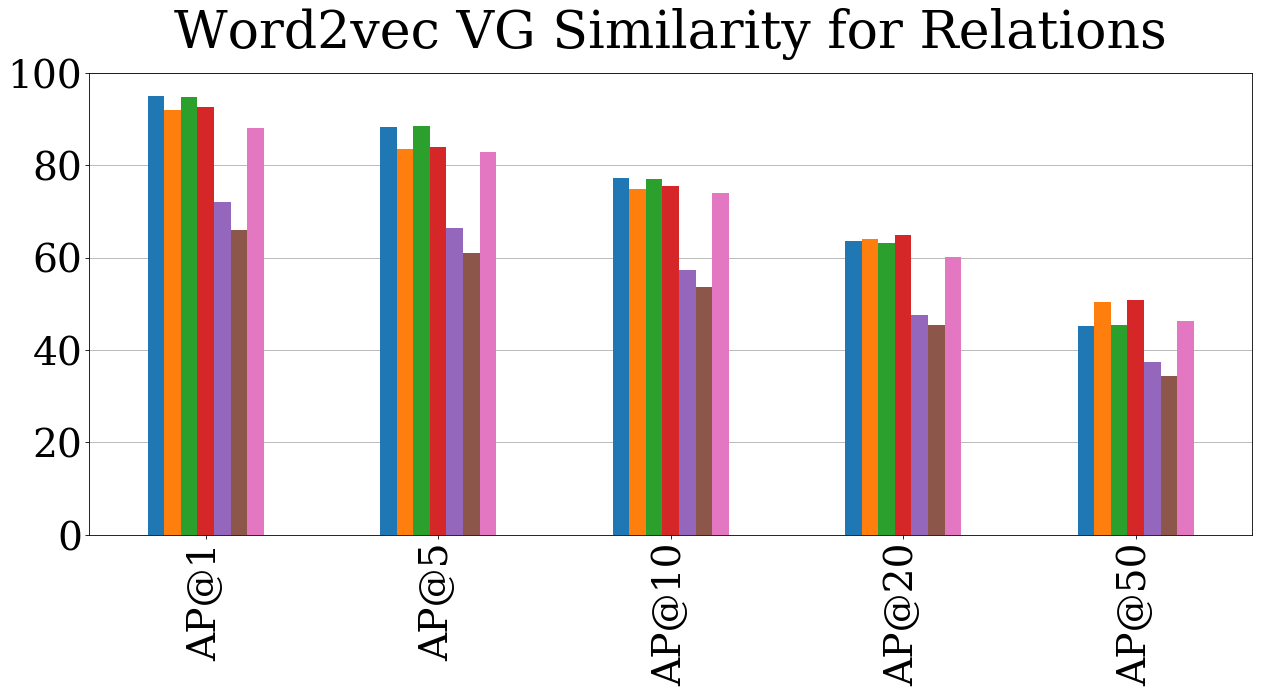}
%   \caption{}
  \label{fig:avg_prec2}
\end{subfigure}
\begin{subfigure}{.3\textwidth}
%   \centering
  \includegraphics[width=\linewidth]{AAAI_supp/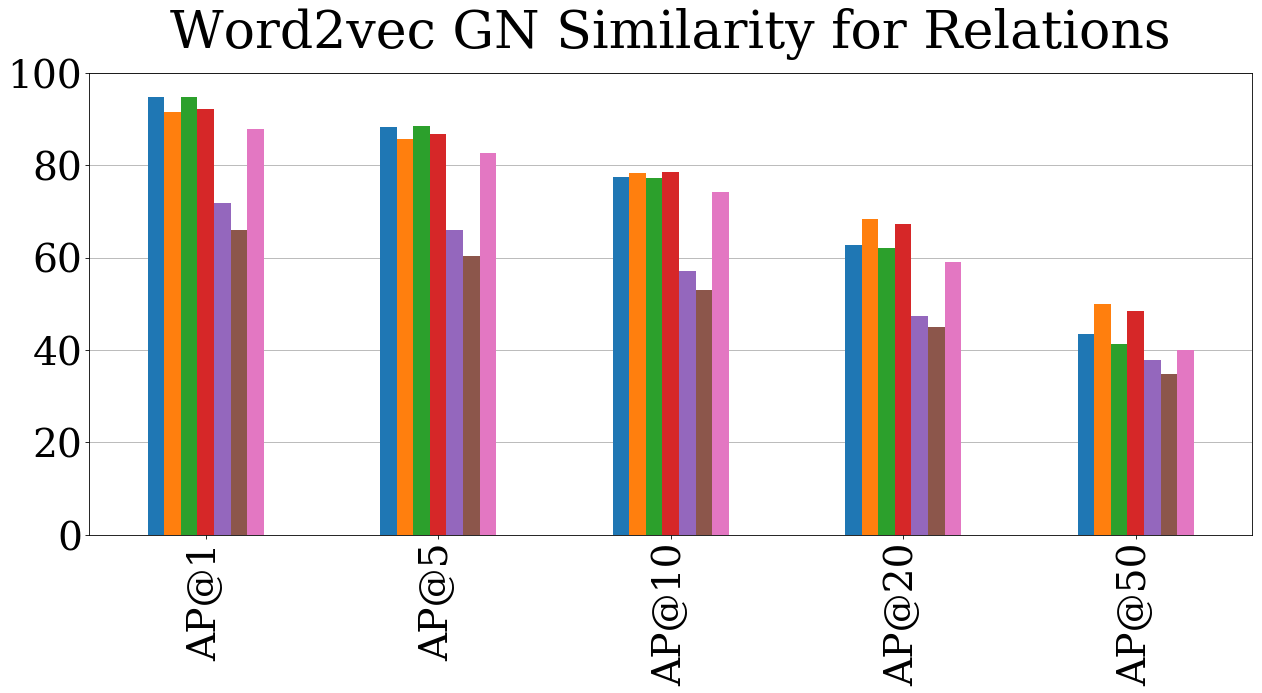}
%   \caption{}
  \label{fig:avg_prec2}
\end{subfigure}
\begin{subfigure}{.3\textwidth}
%   \centering
  \includegraphics[width=\linewidth]{AAAI_supp/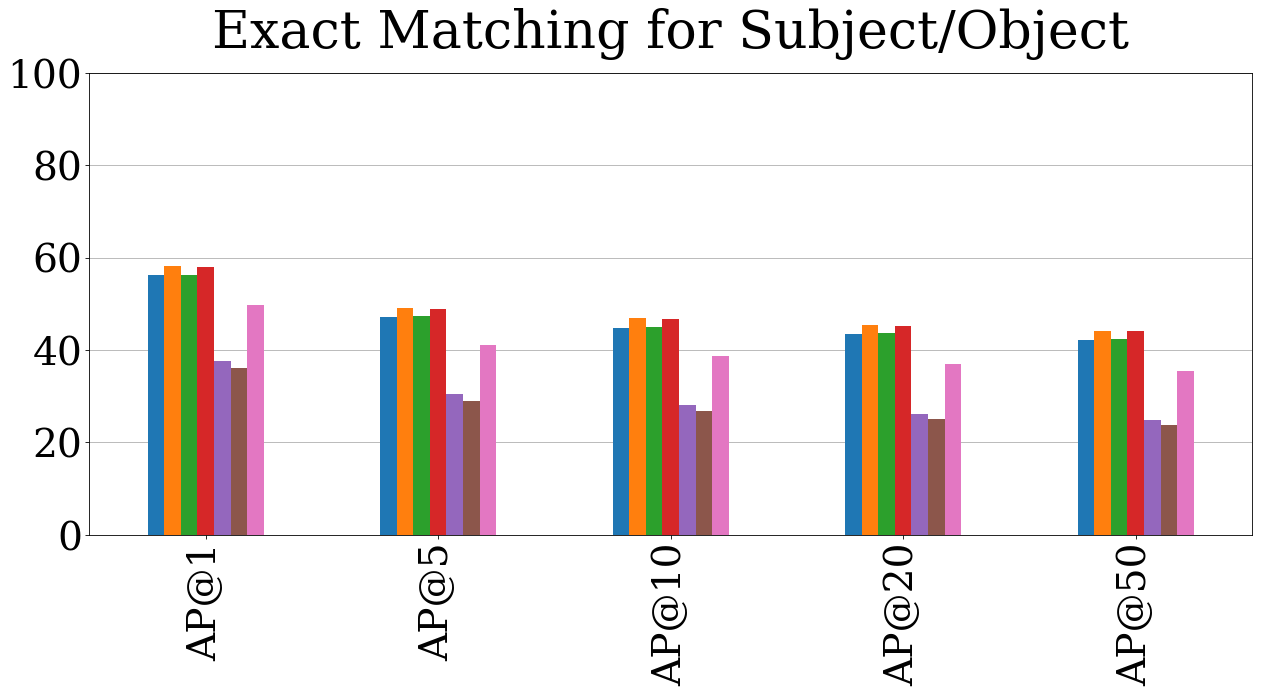}
%   \caption{}
  \label{fig:avg_prec3}
\end{subfigure}%
\begin{subfigure}{.3\textwidth}
%   \centering
  \includegraphics[width=\linewidth]{AAAI_supp/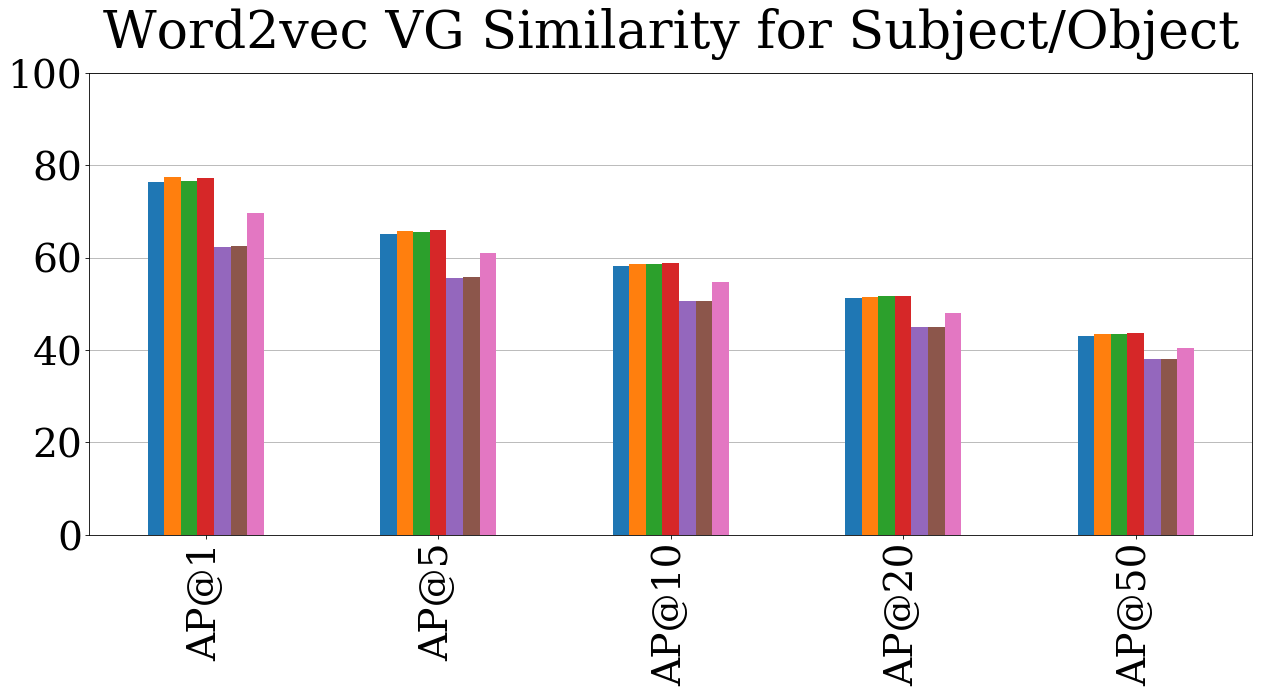}
%   \caption{}
  \label{fig:avg_prec4}
\end{subfigure}
\begin{subfigure}{.3\textwidth}
%   \centering
  \includegraphics[width=\linewidth]{AAAI_supp/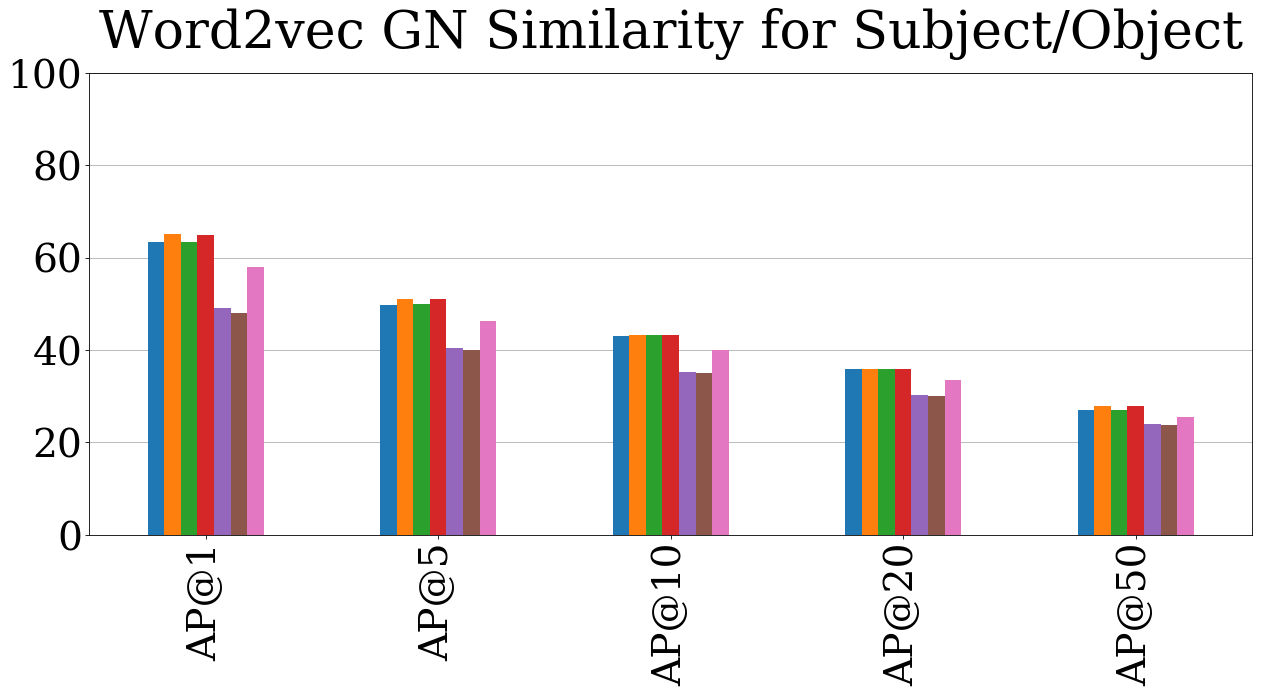}
%   \caption{}
  \label{fig:avg_prec4}
\end{subfigure}
\begin{subfigure}{.3\textwidth}
%   \centering
  \includegraphics[width=\linewidth]{AAAI_supp/figures/average_precision_head/avg_wn_ap_sbj.png}
%   \caption{}
  \label{fig:avg_prec5}
\end{subfigure}

\caption{\textbf{Average precision analysis on the head classes (top 20\% on GQA-LT dataset using a variety of metrics.} We visualize results using exact similarity metrics, W2V-VG, and average of 6 WordNet metrics. The models using VilHub show consistently superior performance on the tail, when compared to similar models without the VilHub.}
\label{fig:avg_prec_head}
\end{figure}

\begin{figure}[h]
\centering
\begin{subfigure}{\textwidth}
  \centering
  \includegraphics[width=.8\linewidth]{AAAI_supp/figures/average_precision_tail/relmix/legend.png}
\end{subfigure}
\begin{subfigure}{.3\textwidth}
%   \centering
  \includegraphics[width=\linewidth]{AAAI_supp/figures/average_precision_tail/relmix/exact_ap_rel.png}
%   \caption{}
  \label{fig:avg_prec1}
\end{subfigure}%
\begin{subfigure}{.3\textwidth}
%   \centering
  \includegraphics[width=\linewidth]{AAAI_supp/figures/average_precision_tail/relmix/w2v_relco_ap_rel.png}
%   \caption{}
  \label{fig:avg_prec2}
\end{subfigure}
\begin{subfigure}{.3\textwidth}
%   \centering
  \includegraphics[width=\linewidth]{AAAI_supp/figures/average_precision_tail/relmix/w2v_ap_rel.png}
%   \caption{}
  \label{fig:avg_prec2}
\end{subfigure}
\begin{subfigure}{.3\textwidth}
%   \centering
  \includegraphics[width=\linewidth]{AAAI_supp/figures/average_precision_tail/relmix/exact_ap_sbj.png}
%   \caption{}
  \label{fig:avg_prec3}
\end{subfigure}%
\begin{subfigure}{.3\textwidth}
%   \centering
  \includegraphics[width=\linewidth]{AAAI_supp/figures/average_precision_tail/relmix/w2v_relco_ap_sbj.png}
%   \caption{}
  \label{fig:avg_prec4}
\end{subfigure}
\begin{subfigure}{.3\textwidth}
%   \centering
  \includegraphics[width=\linewidth]{AAAI_supp/figures/average_precision_tail/relmix/w2v_ap_sbj.png}
%   \caption{}
  \label{fig:avg_prec4}
\end{subfigure}
\begin{subfigure}{.3\textwidth}
%   \centering
  \includegraphics[width=\linewidth]{AAAI_supp/figures/average_precision_tail/relmix/avg_wn_ap_sbj.png}
%   \caption{}
  \label{fig:avg_prec5}
\end{subfigure}

\caption{\textbf{Average precision analysis on the tail classes (bottom 80\% of classes) on GQA-LT dataset using the Relmix approach combined with ViLHub} the figure shows the incremental improvement from adding Relmix augmentation and then ViLHub regularization}
\label{fig:avg_prec_tail_relmix}
\end{figure}

Figure~\ref{fig:avg_prec_head} shows the same analysis done in the main paper section 4.5 Figure 5 but repeated for the head (top 20\% of classes). We can observe the same patterns shown in the main paper, all the models are doing much better than the exact matching metric implies.

Figure~\ref{fig:avg_prec_tail_relmix} shows the average precision analysis for tail classes using the Relmix approach in combination with ViLHub.
% Leacock-Chodorow Similarity(LCH),  
% Wu-Palmer Similarity(WUP), 
% Resnik (RES), 
% Path similarity (PATH), 
% Lin Similarity (LIN),  
% Jiang-Conrath Similarity (JCN)

\section{Further Contrast with Related Work}
\emph{VRD RelationNet}~\cite{dai2017detecting} tackles the problem of VRD, like us, but does not delve into the long-tail nature of the problem. While the method introduced by us $VilHub+RelMix$ is specific for the long-tail task. It also focuses on small scale datasets, while we focus on much larger scale datasets (GQA-LT, VG8K-LT). \emph{Few-shot RelationNet}~\cite{sung2018learning} focuses on the problem of few-shot learning for image recognition and hence the setting is completely different from ours as well.
