# Supplementary material for: Exploring Long Tail Visual Relationship Recognition with Large Vocabulary
Source: arXiv:2004.00436 source file (2021-09-25)
Supplement: Supplementary file 2 [file supp_mat_gvqa_per_class_mean.tex]

% \begin{table*}[ht]
% \begin{center}
% \label{supp:gvqa_cm}
% \begin{tabular}{c||ccc|ccc|ccc}
% Model & Top-1 & Top-5 & Top-10 & Top-1 & Top-5 & Top-10 & Top-1 & Top-5 & Top-10\\
% \hline 
% \hline
% Baseline &15.6\pm0.2 &41.55\pm0.58 &53.49\pm0.39 &15.46\pm0.19 &41.38\pm0.45 &53.29\pm0.26 &2.29\pm0.06 &8.79\pm0.2 &14.15\pm0.45 \\
% Hubness  &15.67\pm0.06 &41.89\pm0.01 &54.25\pm0.56 &15.44\pm0.01 &41.64\pm0.22 &53.97\pm0.42 &2.27\pm0.07 &8.78\pm0.09 &14.28\pm0.14 \\
% Hubness 10K &15.56\pm0.25 &41.5\pm0.01 &53.64\pm0.16 &15.37\pm0.27 &41.20\pm0.17 &53.35\pm0.18 &2.23\pm0.04 &8.66\pm0.3 &14.15\pm0.61 \\
% \hline 
% \end{tabular}
% \caption{\label{tab:avg_per_class_performance} \textbf{Average \textit{per class} performance of different methods.} The numbers are the obtained accuracy for  \textit{object} types (left-most panel),  \textit{subjects} (middle panel) and   \textit{relation} types (right-most panel). Here, we use the accuracy metric for the top-1,5 and 10 model predictions. The results are averages based on 4 random-seeds controlling the network-initialization and the data-set splits.}
% \end{center}
% \end{table*}

\begin{table*}[ht]
\begin{center}
\label{supp:gvqa_cm}
\begin{tabular}{c||cc|cc|cc}
Model & Top-1 & Top-5 & Top-1 & Top-5 & Top-1 & Top-5 \\
\hline 
\hli
Baseline    &15.6\pm0.2     &41.55\pm0.58  &{\bf 15.46}\pm0.19 &41.38\pm0.45 &{\bf 2.29}\pm0.06 &{\bf 8.79}\pm0.2  \\
Hubness     &{\bf 15.67}\pm0.06   &{\bf 41.89}\pm0.01  &15.44\pm0.01 &{\bf 41.64}\pm0.22 &2.27\pm0.07 &8.78\pm0.09 \\
Hubness 10K &15.56\pm0.25   &41.5\pm0.01   &15.37\pm0.27 &41.20\pm0.17 &2.23\pm0.04 &8.66\pm0.3  \\
\hline 
\end{tabular}
\caption{\label{tab:avg_per_class_performance} \textbf{Average \textit{per class} performance of different methods.} The numbers are the obtained accuracy for  \textit{object} types (left-most panel),  \textit{subjects} (middle panel) and   \textit{relation} types (right-most panel). Here, we use the accuracy metric for the top-1, and 5 model predictions. The results are averages based on several random-seeds controlling the network-initialization and the data-set splits.}
\end{center}
\end{table*}
