# Supplementary material for: Exploring Long Tail Visual Relationship Recognition with Large Vocabulary
Source: arXiv:2004.00436 source file (2021-09-25)
Supplement: Supplementary file 3 [file supp_mat_gvqa_simple_mean.tex]

% \begin{table*}[ht]
% \begin{center}
% \label{supp:vgqa_sm}
% \begin{tabular}{c||ccc|ccc|ccc}
% Model & Top-1 & Top-5 & Top-10 & Top-1 & Top-5 & Top-10 & Top-1 & Top-5 & Top-10\\
% \hline 
% \hline
% Baseline &52.08\pm0.28 &81.17\pm0.27 &87.52\pm0.28 &51.64\pm0.28 &80.93\pm0.26 &87.35\pm0.25 &48.87\pm0.06 &97.26\pm0.06 &98.47\pm0.03 \\
% Hubness  &51.89\pm0.15 &80.97\pm0.41 &87.35\pm0.44 &51.46\pm0.16 &80.73\pm0.4 &87.2\pm0.41 &48.92\pm0.06 &97.22\pm0.06 &98.47\pm0.03  \\
% Hubness 10K &52.02\pm0.28 &81.04\pm0.27 &87.46\pm0.22 &51.59\pm0.29 &80.82\pm0.28 &87.31\pm0.22 &48.88\pm0.06 &97.24\pm0.04 &98.47\pm0.01 \\
% \hline 
% \end{tabular}
% \caption{\label{tab:avg_per_class_performance} \textbf{Average performance of different methods.} The numbers are the obtained accuracy for  \textit{object} types (left-most panel),  \textit{subjects} (middle panel) and   \textit{relation} types (right-most panel). Here, we use the accuracy metric for the top-1,5 and 10 model predictions. The results are averages based on 4 random-seeds controlling the network-initialization and the data-set splits.}
% \end{center}
% \end{table*}

\begin{table*}[ht]
\begin{center}
\label{supp:vgqa_sm}
\begin{tabular}{c||cc|cc|cc}
Model & Top-1 & Top-5 & Top-1 & Top-5 & Top-1 & Top-5\\
\hline 
\hline
Baseline    &{\bf 52.08}\pm0.28   &{\bf 81.17}\pm0.27   &{\bf 51.64}\pm0.28   &{\bf 80.93}\pm0.26    &48.87\pm0.06 &{\bf 97.26}\pm0.06 \\
Hubness     &51.89\pm0.15   &80.97\pm0.41   &51.46\pm0.16   &80.73\pm0.4     &{\bf 48.92}\pm0.06 &97.22\pm0.06  \\
Hubness 10K &52.02\pm0.28   &81.04\pm0.27   &51.59\pm0.29   &80.82\pm0.28    &48.88\pm0.06 &97.24\pm0.04 \\
\hlin
\end{tabular}
\caption{\label{tab:avg_per_class_performance} \textbf{Average performance of different methods.} The numbers are the obtained accuracy for  \textit{object} types (left-most panel),  \textit{subjects} (middle panel) and   \textit{relation} types (right-most panel). Here, we use the accuracy metric for the top-1, and 5 model predictions. The results are averages based on several random-seeds controlling the network-initialization and the data-set splits.}
\end{center}
\end{table*}
