# Supplementary material for: Exploring Long Tail Visual Relationship Recognition with Large Vocabulary
Source: arXiv:2004.00436 source file (2021-09-25)
Supplement: Supplementary file 4 [file supp_mat_vg_per_class_mean.tex]

% \begin{table*}[ht]
% \begin{center}
% \label{supp:vg_cm}
% \begin{tabular}{c||ccc|ccc|ccc}
% Model & Top-1 & Top-5 & Top-10 & Top-1 & Top-5 & Top-10 & Top-1 & Top-5 & Top-10\\
% \hline 
% \hline
% Baseline &5.71\pm0.18 &18.12\pm0.51 &25.69\pm1.04 &5.27\pm0.27 &16.75\pm0.63 &23.41\pm0.71 &0.37\pm0.02 &2.044\pm0.05 &3.78\pm0.07 \\
% Hubness  &5.79\pm0.28 &18.25\pm0.69 &25.54\pm1.19 &5.35\pm0.25 &17.01\pm0.79 &23.62\pm0.90 &0.38\pm0.02 &2.04\pm0.12 &3.69\pm0.04 \\
% Hubness 10K &5.84\pm0.12 &18.17\pm0.38 &25.78\pm0.39 &5.45\pm0.16 &17.05\pm0.22 &23.89\pm0.56 &0.37\pm0.01 &2.09\pm0.04 &3.77\pm0.13 \\
% \hline 
% \end{tabular}
% \caption{\label{tab:avg_per_class_performance} \textbf{Average \textit{per class} performance of different methods.} The numbers are the obtained accuracy for  \textit{object} types (left-most panel),  \textit{subjects} (middle panel) and   \textit{relation} types (right-most panel). Here, we use the accuracy metric for the top-1,5 and 10 model predictions. The results are averages based on 4 random-seeds controlling the network-initialization and the data-set splits.}
% \end{center}
% \end{table*}

\begin{table*}[ht]
\begin{center}
\label{supp:vg_cm}
\begin{tabular}{c||cc|cc|cc}
Model & Top-1 & Top-5  & Top-1 & Top-5  & Top-1 & Top-5 \\
\hline 
\hline
Baseline        &5.71\pm0.18 &18.12\pm0.51  &5.27\pm0.27 &16.75\pm0.63  &0.37\pm0.02 &2.044\pm0.05  \\
Hubness         &5.79\pm0.28 &{\bf 18.25}\pm0.69  &5.35\pm0.25 &17.01\pm0.79  &{\bf 0.38}\pm0.02 &2.04\pm0.12   \\
Hubness 10K     &{\bf 5.84}\pm0.12 &18.17\pm0.38  &{\bf 5.45}\pm0.16 &{\bf 17.05}\pm0.22  &0.37\pm0.01 &{\bf 2.09}\pm0.04   \\
\hline 
\end{tabular}
\caption{\label{tab:avg_per_class_performance} \textbf{Average \textit{per class} performance of different methods.} The numbers are the obtained accuracy for  \textit{object} types (left-most panel),  \textit{subjects} (middle panel) and   \textit{relation} types (right-most panel). Here, we use the accuracy metric for the top-1, and 5 model predictions. The results are averages based on several random-seeds controlling the network-initialization and the data-set splits.}
\end{center}
\end{table*}
