# Supplementary material for: Exploring Long Tail Visual Relationship Recognition with Large Vocabulary
Source: arXiv:2004.00436 source file (2021-09-25)
Supplement: Supplementary file 5 [file supp_mat_vg_simple_mean.tex.tex]

% \begin{table*}[ht]
% \begin{center}
% \label{supp:vg_sm}
% \begin{tabular}{c||ccc|ccc|ccc}
% Model & Top-1 & Top-5 & Top-10 & Top-1 & Top-5 & Top-10 & Top-1 & Top-5 & Top-10\\
% \hline 
% \hline
% Baseline &50.89\pm0.49 &77.06\pm0.4 &82.91\pm0.44 &48.24\pm0.38 &74.15\pm0.4 &80.5\pm0.28 &53.08\pm0.29 &79.67\pm0.1 &85.65\pm0.07 \\
% Hubness  &50.71\pm0.18 &76.9\pm0.23 &82.62\pm0.25 &48.3\pm0.26 &74.1\pm0.2 &80.32\pm0.2 &52.68\pm0.23 &79.62\pm0.1 &85.58\pm0.07 \\
% Hubness 10K &51.04\pm0.2 &77.31\pm0.29 &83.07\pm0.29 &48.71\pm0.2 &74.59\pm0.29 &80.89\pm0.27 &52.88\pm0.43 &79.68\pm0.16 &85.7\pm0.075 \\
% \hline 
% \end{tabular}
% \caption{\label{tab:avg_per_class_performance} \textbf{Average performance of different methods.} The numbers are the obtained accuracy for  \textit{object} types (left-most panel),  \textit{subjects} (middle panel) and   \textit{relation} types (right-most panel). Here, we use the accuracy metric for the top-1,5 and 10 model predictions. The results are averages based on 4 random-seeds controlling the network-initialization and the data-set splits.}
% \end{center}
% \end{table*}

\begin{table*}[ht]
\begin{center}
\label{supp:vg_sm}
\begin{tabular}{c||cc|cc|cc}
Model & Top-1 & Top-5 & Top-1 & Top-5 & Top-1 & Top-5\\
\hline 
\hline
Baseline    &50.89\pm0.49   &77.06\pm0.4    &48.24\pm0.38   &74.15\pm0.4    &{\bf 53.08}\pm0.29 &79.67\pm0.1  \\
Hubness     &50.71\pm0.18   &76.9\pm0.23    &48.3\pm0.26    &74.1\pm0.2     &52.68\pm0.23 &79.62\pm0.1  \\
Hubness 10K &{\bf 51.04}\pm0.2    &{\bf 77.31}\pm0.29   &{\bf 48.71}\pm0.2    &{\bf 74.59}\pm0.29   &52.88\pm0.43 &{\bf 79.68}\pm0.16 \\
\hline 
\end{tabular}
\caption{\label{tab:avg_per_class_performance} \textbf{Average performance of different methods.} The numbers are the obtained accuracy for  \textit{object} types (left-most panel),  \textit{subjects} (middle panel) and   \textit{relation} types (right-most panel). Here, we use the accuracy metric for the top-1,and 5model predictions. The results are averages based on several random-seeds controlling the network-initialization and the data-set splits.}
\end{center}
\end{table*}
